# Supplementary material for: Benchmarking Deep Reinforcement Learning for Continuous Control
Source: arXiv:1604.06778 source file (2016-05-27)
Supplement: Supplementary file 1 [file appendix.tex]

\section{Supplementary}
\subsection{Tasks}
\subsubsection{Basic Tasks}

{\bf Cart-Pole Balancing}: The observation consists of the cart position, pole angle ($\theta$), and their respective velocities. The 1D action consists of the horizontal force applied to the cart body. The reward function is given by 
$r(s, a) := 10 - (1 - \cos(\theta)) - 10^{-5} \norm{a}_2^2$. The episode terminates when the cart moves too far away from the origin or if $\theta$ deviates too much from its original value.

{\bf Cart-Pole Swing Up}: A slightly more complex version of the previous task has been proposed by \citet{815604} in which the system should not only be able to balance the pole, but first succeed in swinging it up into an upright position. Except for the initial pole position, which now points downwards, the observations, actions, and dynamics remain the same. The reward function is given by $r(s, a) := \cos(\theta)$. The episode terminates when the cart moves too far away from the origin, accompanied by negative reward of $-100$.

{\bf Mountain Car}: We implement a continuous version of the classic task described in \citet{Moore90MountainCar}. The observation is composed of the horizontal position and velocity of the car, while the reward is given by $r(s, a) := -1 + \textrm{height}$, with $\textrm{height}$ the car's vertical offset. As an episode only terminates when the car reaches a target height, the goal is to it in minimal time.

{\bf Acrobot Swing Up}: We use the same physics parameters as in \citet{Sutton98RLBook}. The observation includes the two joint angles and their velocities, while the action consists of the torques applied at the two joints. The reward is defined as $r(s, a) := -\norm{\mathrm{tip}(s) - \mathrm{tip}_{\mathrm{target}}}_2$, where $\mathrm{tip}(s)$ computes the Cartesian position of the tip of the robot given the joint angles.

{\bf Double Inverted Pendulum Balancing}: Our implementation is based on the design of \citet{Furuta78}. The observation includes the cart position, joint angles ($\theta_{1,2}$), and joint velocities ($\dot\theta_{1,2}$). We encode each joint angle as its sine and cosine values. The action is the same as in cart-pole tasks. The reward is given by $r(s, a) = 10 - 0.01 x_{\mathrm{tip}}^2 - (y_{\mathrm{tip}} - 2)^2 - 10^{-3} \cdot \dot\theta_1^2 - 5\cdot 10^{-3} \cdot \dot\theta_2^2$, where $x_{\mathrm{tip}}, y_{\mathrm{tip}}$ are the coordinates of the tip of the pole.

\subsubsection{Locomotion Tasks}

We implement six (\todo simple/humanoid same task?) locomotion tasks, using MuJoCo \cite{MuJoCo} for its better modeling of contact dynamics.
%%PA: "for fast simulation" is a bit brief.  People might argue with this / not be convinced it's indeed the simulator to pick for fast simulation;  ideally there would be a good argument as to why we use MuJoCo, but short of a good argument, no argument might be better than a not-so-great one
%%PA: none of the tasks below have citations -- most of them have been proposed before though, right?  it's important to give credit here to the original papers (and maybe not only the original papers, but also some other papers who have contributed to popularizing a certain task)

{\bf Swimmer}: This is a planar robot with 13-dim observations and 2-dim actions. The reward is given by $r(s, a) = v_x - 0.005 \norm{a}_2^2$, where $v_x$ is the forward velocity.

%3 links, using viscosity forces to simulate simple fluid dynamics. The reward is given by

{\bf Hopper}: This is a planar monopod robot with 20-dim observations and 3-dim actions. The reward is given by
$r(s, a) := v_x - 0.005 \cdot \norm{a}_2^2 + 1$,
where the last term is a bonus for being ``alive.'' The episode is terminated when the head is too low, or when the body is falling down.

{\bf Walker}: This is a planar biped robot with 21-dim observations and 6-dim actions. The reward is given by
$r(s, a) := v_x - 0.005 \cdot \norm{a}_2^2$.
The episode is terminated when the head is too low or too high, or when the body is falling down.

{\bf Half-Cheetah}: This is a planar biped robot with 20-dim observations and 6-dim actions. The reward is given by
$r(s, a) = v_x - 0.05 \cdot \norm{a}_2^2$.

{\bf Ant}: This is a 3D quadruped robot with 125-dim observations and 8-dim actions, where we have a high-dimensional observation due to the inclusion of a sparse vector of constraint forces. The reward is given by $r(s, a) = v_x - 0.005 \cdot \norm{a}_2^2 - C_{\mathrm{contact}} + 0.05$, where $C_{\mathrm{contact}}$ penalizes contacts to the ground, and is given by
$5\cdot 10^{-4} \cdot \norm{F_{\mathrm{contact}}}_2^2$, where $F_{\mathrm{contact}}$ is the contact force vector clipped to values between $-1$ and $1$.

{\bf Simple Humanoid}: This is a simplified 3D humanoid robot with 102-dim observations and 10-dim actions. The reward is given by
$r(s, a) = v_x - 5\cdot 10^{-4} \norm{a}_2^2 - C_{\mathrm{contact}} - C_{\mathrm{deviation}} + 0.2$, where $C_{\mathrm{contact}} = 5\cdot 10^{-6} \cdot \norm{F_{\mathrm{contact}}}$, and $C_{\mathrm{deviation}} = 5\cdot 10^{-3} \cdot (v_y^2 + v_z^2)$ to penalize deviation from the forward direction.

{\bf Full Humanoid}: This is a 3D humanoid robot with 142-dim observations and 21-dim actions, including more details than the simple humanoid. The same reward function is used as in the simple humanoid model.
